# Supplementary material for: Global Fits in the Supersymmetric Georgi-Machacek Model
Source: arXiv:2408.04489 source file (2024-08-08)
Supplement: Supplementary file 1 [file appendixBfits.tex]

\begin{singlespace}
\chapter{The Monte Carlo Analysis}\label{appendix:}
\end{singlespace}

\section{The Bayesian Framework}

Consider a model $M$ with some parameters $\vec{\lambda}$. Let $\vec{x}$ be some predictions from the model $M$ and $\vec{D}$ be some measured data points. The posterior distribution, which contains the information of the model $M$ after the experiment is analyzed, is \begin{equation}
P(\vec{\lambda}, M \mid \vec{D})=\frac{f(\vec{x}=\vec{D} \mid \vec{\lambda}, M) P_0(\vec{\lambda}, M)}{\sum_M \int f(\vec{x}=\vec{D} \mid \vec{\lambda}, M) P_0(\vec{\lambda}, M) d \vec{\lambda}},
\end{equation}
where $P_0$ is the prior distribution of $\vec{\lambda}$, which contains all the information of the model before the experiment is performed. $f$, an unnormalized probability density function, is viewed as a relative frequency of a particular outcome $\vec{x}=\vec{D}$. It is known as the likelihood. The denominator is called normalization for evidence. It is the probability to get data $\vec{D}$ assuming model $M$. Since $f$ is normalized, we can write \begin{equation}
P(\vec{D} \mid \vec{\lambda}, M)=f(\vec{x}=\vec{D} \mid \vec{\lambda}, M).
\end{equation}
Thus, Eq. (B.2.1) is simply the Bayes' theorem: \begin{equation}
P(\vec{\lambda}, M \mid \vec{D})=\frac{P(\vec{D} \mid \vec{\lambda}, M) P(\vec{\lambda}, M)}{P(\vec{D})}.
\end{equation}
For individual parameters, we can compute the marginalized posterior distribution for $\lambda_i$ by \begin{equation}
P\left(\lambda \mid \vec{D}\right)=\int P(\vec{\lambda},M \mid D) \prod_{j \neq i} d \lambda_j,
\end{equation}
where all model parameters except the one for which the marginalized distribution is computed are integrated over, and this can be generalized to more parameters. 

\section{Markov Chain Monte Carlo Simulation}

Markov chains are sequences of random numbers $X_t$, which have a well-defined limiting distribution $\pi(x)$. In a Markov chain, the probability distribution of a element $X_{t+1}$ depends only on the current state, not on any previous history. Thus, it is completely defined by the one step probability transition matrix $P(X_{t+1}=x_{t+1}\mid X_t=x_t)$. A Markov chain Monte Carlo is a method of  producing an ergodic Markov chain, where the stationary distribution is the distribution of interest, i.e. $\pi=P(\vec{\lambda} \mid \vec{D}, M)$\cite{Caldwell:2008fw}. The \texttt{BAT} package embedded in \texttt{HEPfit} uses a Metropolis-Hastings algorithm to sample the parameter space from the posterior. Given a probability density function $f$, the Metropolis-Hastings algorithm starts with a random point $\vec{x}$ in the parameter space. It then generate a proposal point $\vec{y}$ according to a symmetric distribution $g(\vec{x},\vec{y}$. The proposal point is accepted if \begin{equation}
f(\vec{y}) \geq f(\vec{x}), \quad f(\vec{y}) / f(\vec{x})>r,
\end{equation}
where $r\in(0,1)$ is a random number. This process is then repeated.
