# Supplementary material for: Global Fits in the Supersymmetric Georgi-Machacek Model
Source: arXiv:2408.04489 source file (2024-08-08)
Supplement: Supplementary file 2 [file appendixC.tex]

\begin{singlespace}
\chapter{}\label{appendix:}
\end{singlespace}
